# Supplementary material for: Detection of single ions in a nanoparticle coupled to a fiber cavity
Source: arXiv:2303.00017 ancillary file (2023-02-28)
Supplement: Supplementary file 1 [file Single_Er_Ions_SM.pdf]

# Supplementary Material for: Detection of single ions in a nanoparticle coupled to a fiber cavity

Chetan Deshmukh,[1] Eduardo Beattie,[1] Bernardo Casabone,[1] Samuele Grandi,[1] Diana Serrano,[2] Alban Ferrier,[2,3] Philippe Goldner,[2] David Hunger,[4,5] and Hugues de Riedmatten[1,6]

[1]*ICFO-Institut de Ciencies Fotoniques, The Barcelona Institute of Science and Technology, 08860 Castelldefels (Barcelona), Spain.*

[2]*Chimie ParisTech, PSL University, CNRS, Institut de Recherche de Chimie Paris, Paris, France.*

[3]*Faculté des Sciences et Ingénierie, Sorbonne Université, UFR 933, 75005 Paris, France*

[4]*Karlsruher Institut für Technologie, Physikalisches Institut, Karlsruhe, Germany.*

[5]*Karlsruhe Insitute for Technology, Institute for Quantum Materials and Technologies (IQMT), Eggenstein-Leopoldshafen, Germany.*

[6]*ICREA-Institució Catalana de Recerca i Estudis Avançats, 08015 Barcelona, Spain.*

## DETECTION OF INDIVIDUAL SPECTRAL LINES

During the course of the experiment we performed several scans of the inhomogeneous broadening of nanoparticles. We report here a fluorescence excitation scan performed on a different nanoparticle from that reported in the main text. Fig. 1 shows counts received per excitation cycle as a function of laser frequency detuning from 1535.49 nm. The scan covers a detuning range of 5 to 30 GHz and we can clearly identify three distinct spectral features within this range. The widths of these peaks are larger than expected for these temperature, possibly due to an imperfect cooling of this nanoparticle, or a sub-optimal positioning within the nanocrystal.

## ADDITIONAL CROSS-CORRELATION MEASUREMENT

We report here another cross-correlation measurement taken on the spectral feature labelled as "ion 1" in Fig. 1. We measured the $g^{(2)}(\tau)$ of the emitted photons by performing a Hanbury Brown-Twiss (HBT) experiment, but with two detectors (in the main text, only one detector was used). We considered only the initial 200 $\mu$s of the detection window, where the signal count-rate is estimated to be $\sim$18 Hz per detector, which corresponds to a signal-to-noise ratio (SNR) of $\sim 2$ in each detector in this window. The results are reported in Fig. 2. We can calculate the value of $g^{(2)}(0) = 0.59(5)$, which is close to the value we would expect given SNR = 2. As this value is already below 1, the input photonic state can already be classified as non-classical, which is strong evidence for the single emitter nature of the spectral feature. The orange dotted line in Fig. 2 indicates the expected background coincidences due to the presence of noise. It includes contributions from coincidences between signal-noise as well as noise-noise. Subtracting the background coincidences gives a corrected value of $g^{(2)}(0) = 0.29(9)$. Emission from other detuned ions, such as Ion 2 (see Fig. 1), could be limiting the corrected value from reaching 0. We have also occasionally detected bursts of additional counts, which originate from the coupling of electronic noise to our detectors, that could be contributing to the coincidences in the same trial. For the data presented in Fig. 4 of the main text, the signal-to-noise was increased by using only one detector, and by lowering the efficiency, which greatly reduced the dark count rate.

## SPECTRAL DIFFUSION

Besides the spectral diffusion measurements reported in Fig. 3(a) of the main text, we ran longer tests to check the stability of the ion. During these measurements, the excitation light was repeatedly switched between the different frequencies probed every 200 ms in random order to ensure equal sampling for all frequencies at all times. One such measurement is reported in Fig. 3, where no magnetic field was present and where the ion is stable for over 200 minutes. A few bright lines are also visible in the plot, crossing the resonance frequency of the ion. We believe these to be other erbium ions, diffusing fast over a wide range. Occasionally we observed considerably worse stability for limited period of times, where the central frequency changed by up to a few linewidths, but eventually returned to a stable configuration. A potential explanation for this behaviour could be a change in the local electric environment, due for example to local surface charges.

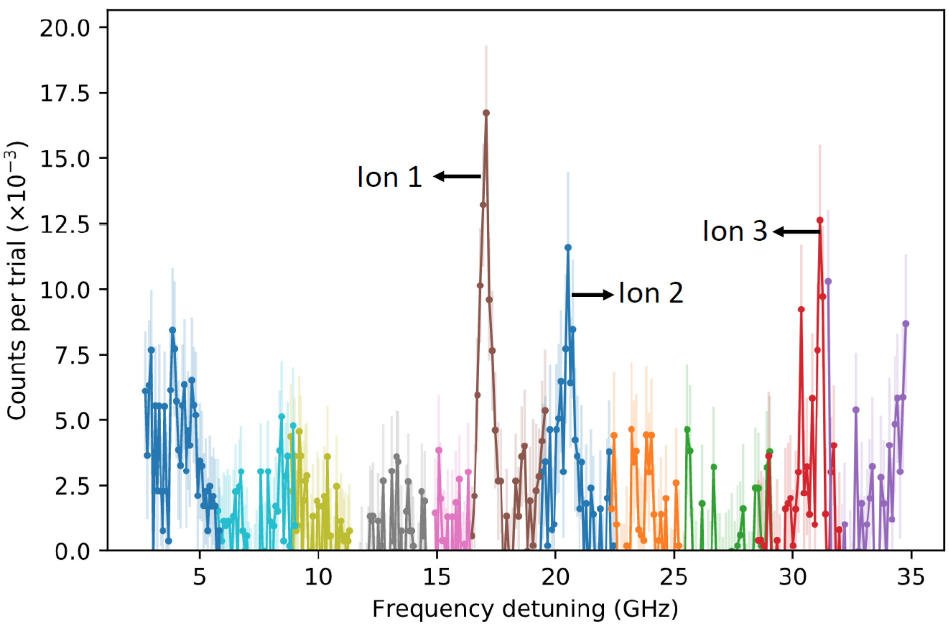


Figure 1: Counts received per trial as a function of laser frequency detuning from 1535.49 nm. Colours represent scans done in different spectral regions. Three features are labelled.

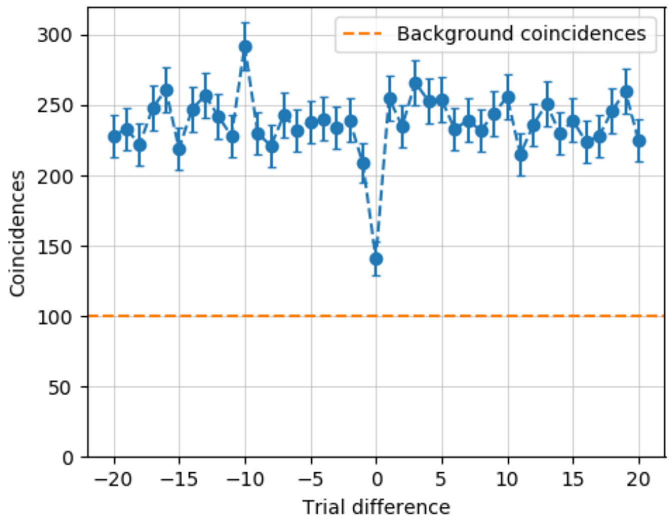


Figure 2: Coincidence counts as a function of trial difference. Orange dotted line indicates the expected background coincidences due to the presence of noise. We calculate an uncorrected $g^{(2)}(0) = 0.59(5)$, which after background subtraction gives $g^{(2)}(0) = 0.29(9)$.

## SYSTEM EFFICIENCY

As mentioned in the main text, the probability to detect a photon per trial at saturation approaches $p_{\max} = 1\%$. This value includes several system efficiencies:

- the probability $\eta_{\text{exc}} = 50\%$ of exciting an ion with resonant light;
- the probability $\eta_{\text{match}}$ of emission of a photon in the mode of the cavity and its coupling to that of the fiber;
- the transmission $\eta_{\text{T}}$ of the optical setup from the cavity to the detector;
- the detection efficiency $\eta_{\text{det}}$, given a specific detection window.

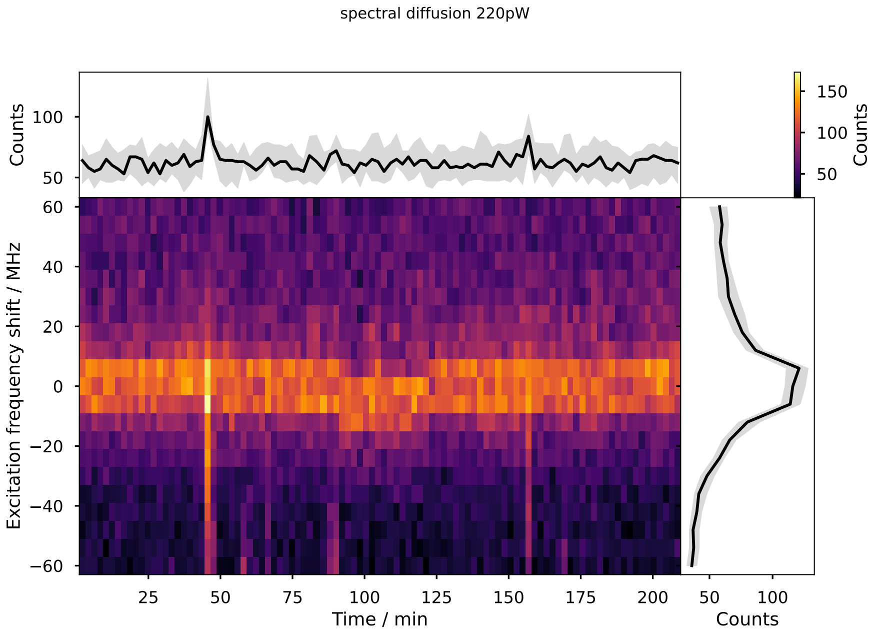


Figure 3: Spectrum of a single ion showing stability over 200 minutes. The emission center drifts by just $1.3 \pm 4.0$ MHz between the initial and final spectra, and the linewidth calculated from the accumulated counts is 30(6) MHz. The RMS drift of the emission center is 4.0 MHz. The adjacent plots show the median and inter-quartile ranges of the data for each frequency and time bin.

The detection efficiency of the superconducting detectors is $\eta_{\mathrm{det}} = 80\%$, and the transmission $\eta_{\mathrm{T}}$ was measured to be $\sim 44\%$. $\eta_{\mathrm{det}}$ has to be reduced to 53%, due to the reduced detection window (500 $\mu s$) which limited the count rate. We can then estimate the probability of having a photon in the fibre after an excitation attempt as $p_{\mathrm{f}} \approx 4.3\%$. From the cavity parameters and the intra-cavity loss due to the nanoparticle we can estimate the escape efficiency of a photon from the curved mirror to be 32%, which implies a mode-matching of 25% between the mode of the cavity and the mode of the fibre. This is lower than anticipated from the geometry of the cavity (71%), and its reduction is still under investigation.

One factor that we haven't considered so far is related to population shelving in the Zeeman states, after the line is split. We believe that the Zeeman states lifetime is well-below the length of our excitation path due to the lack of bunching in the cross-correlation measurement and from saturation traces for the ion with and without magnetic field, which saturate to a similar maximum detection probability.

## FLUORESCENCE DECAY OF THE ION

The data that was gathered during the cross-correlation measurement shown in Fig. 4 of the main text can be analysed to obtain the lifetime of the ion. Due to the pulsed excitation regime, correlating the detected count with the excitation trigger shows an exponential decay of the fluorescence, with a decay constant equal to the lifetime. The result is reported in Fig. 4, where the data perfectly overlaps with the fit. It is then possible to see that the width of the detection window affects the final detection efficiency, since the fluorescence extends beyond the 500 $\mu$s window used in the main text for the power saturation measurement.

The decay constant in this case it 467 $\mu$s, higher than the lifetime initially reported for this ion, which was around 350 $\mu$s. This is due to a slow increase in the vibration that our cryostat (Montana Instruments Cryostation) imparted on the nanopositioner. Initial condition could be recovered by readjusting the vibration isolation system, a demanding procedure which we elected not to perform. Employing a more stable cryostat, one with an exchange gas environment for example, could improve this stability.

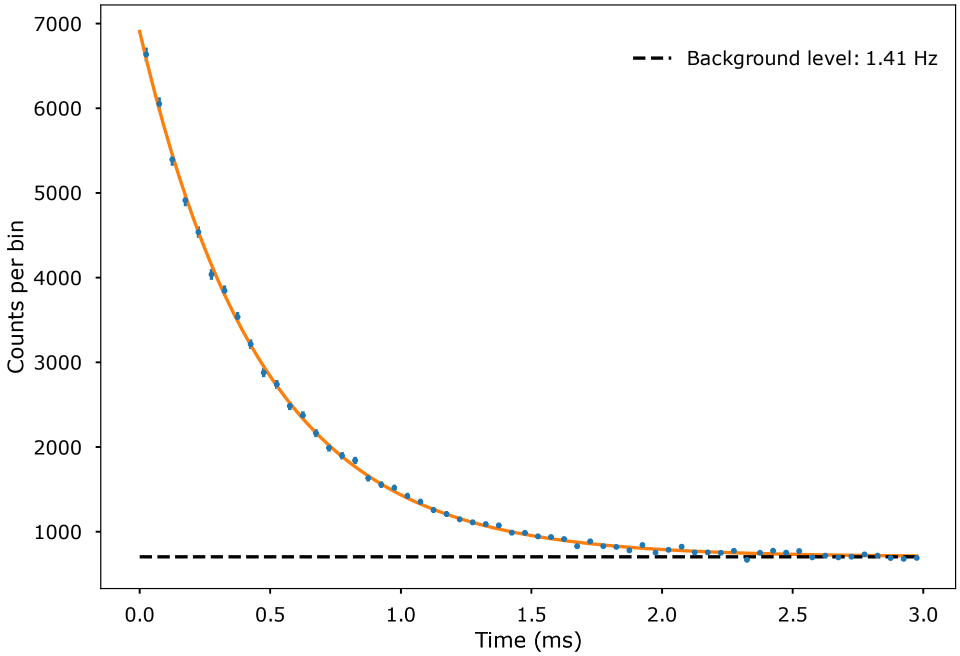


Figure 4: Fluorescence decay measurement for the ion analyzed in the main text. The data is the same used to calculate the auto-correlation function reported in Fig. 4 of the main text.
